# Supplementary material for: LegalViz: Legal Text Visualization by Text To Diagram Generation
Source: arXiv:2502.06147 source file (2025-02-13)

(A) Gemma2-9B ft.

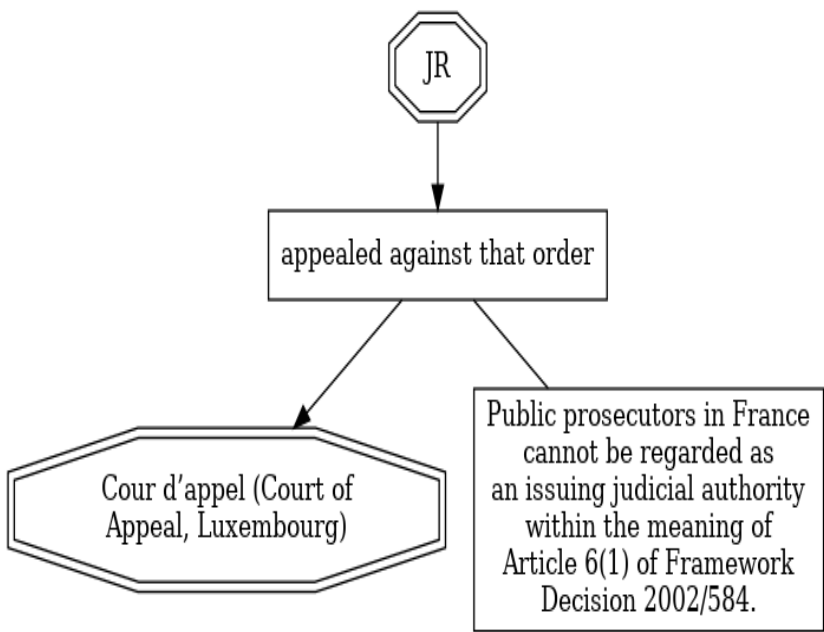

(B) CodeLlama-13B it. ft.

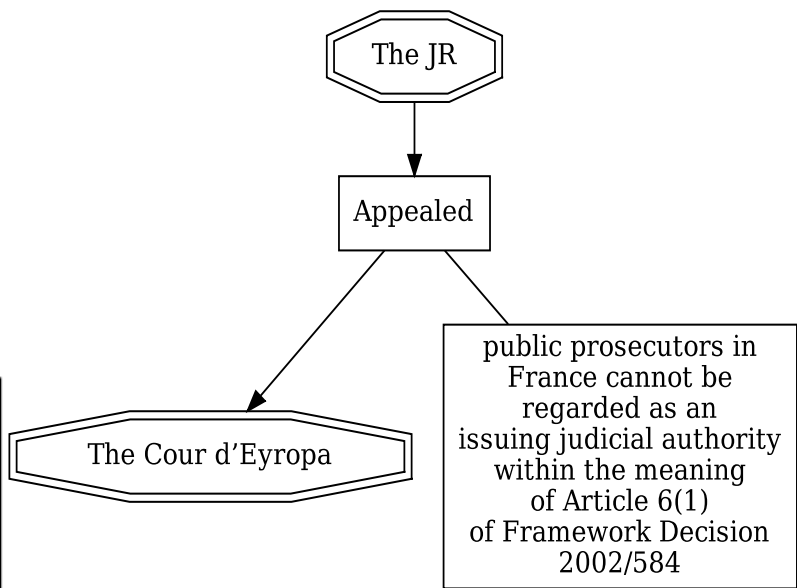

(C) GPT-3.5-Turbo

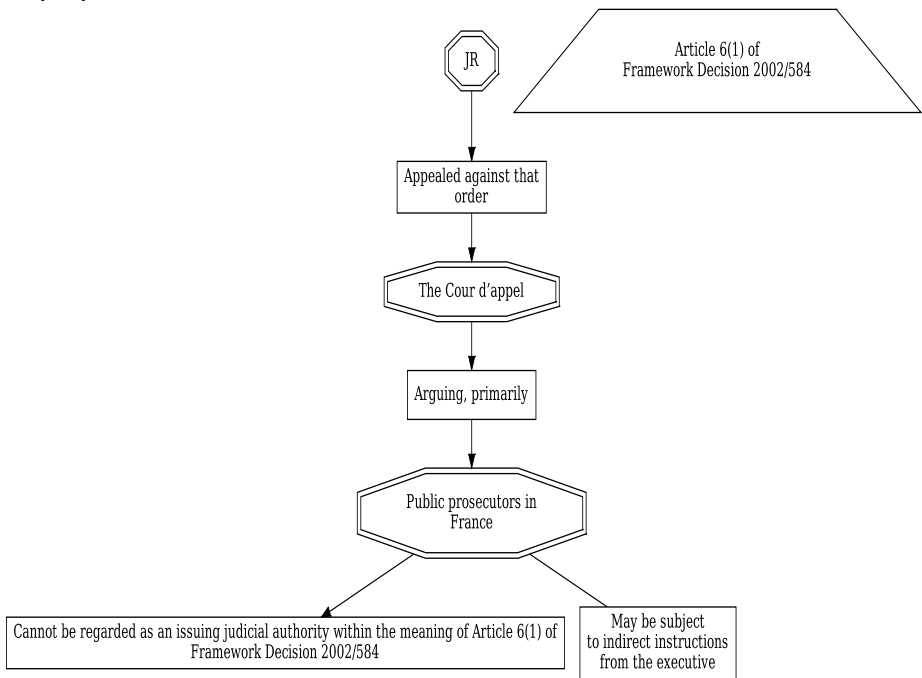

(D) GPT-4

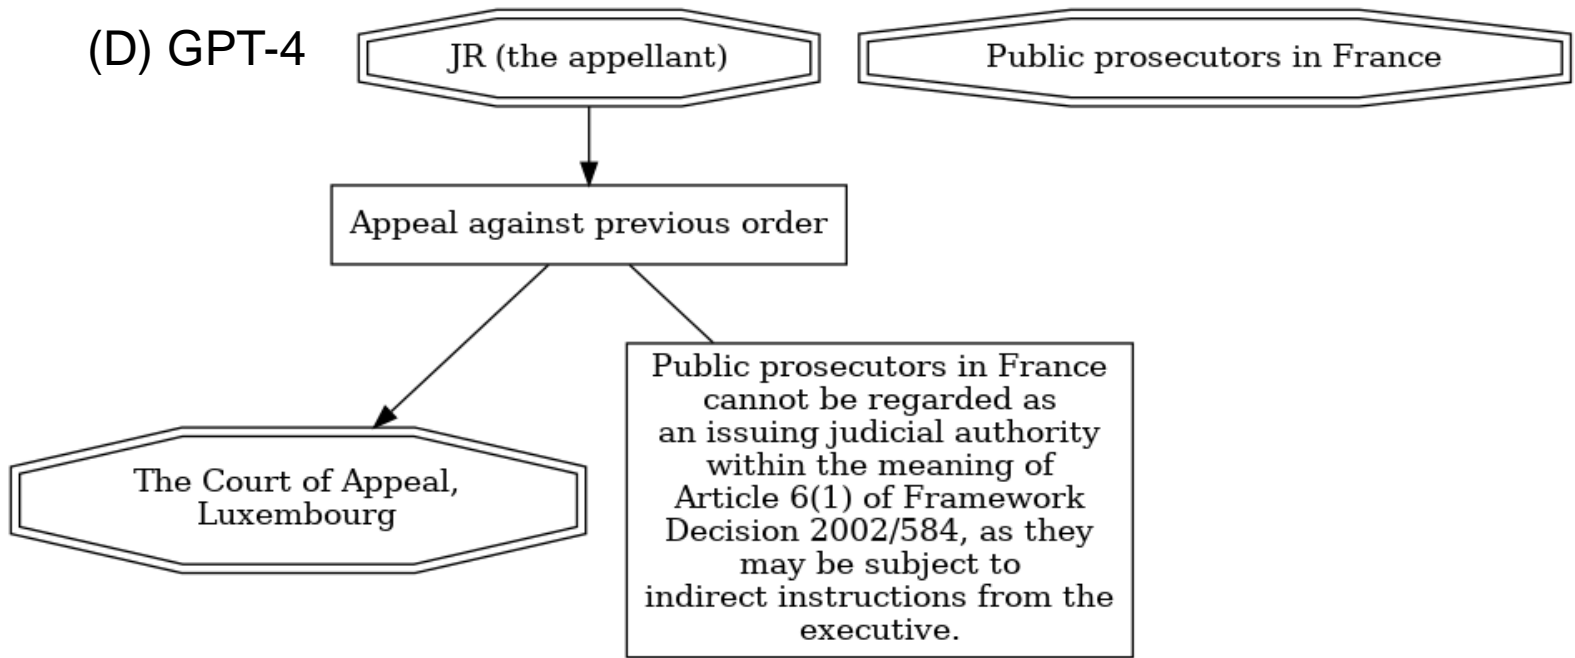

(E) Annotated

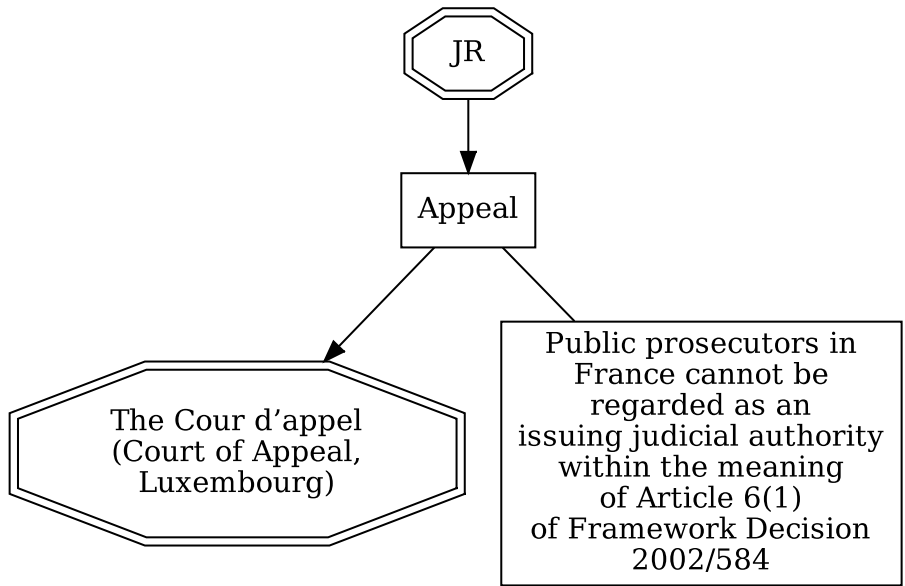

(E) Annotated

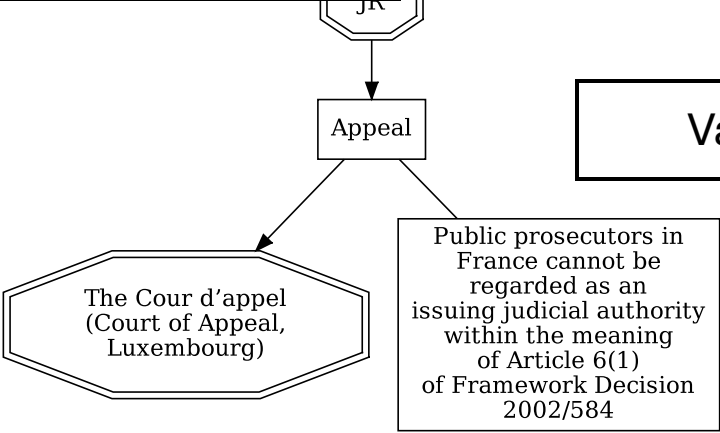

CodeLlama13b t. Ft.

Valid-1280

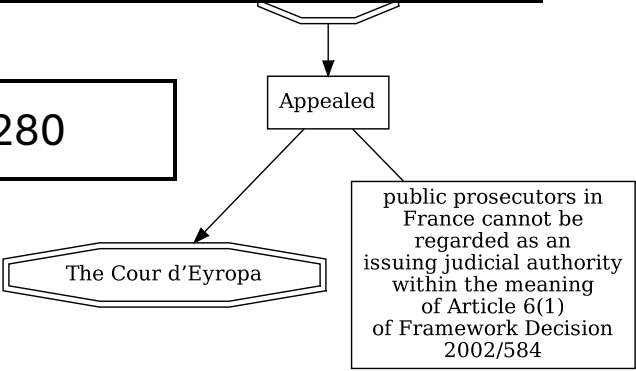

(A) Gemma2-9B ft.

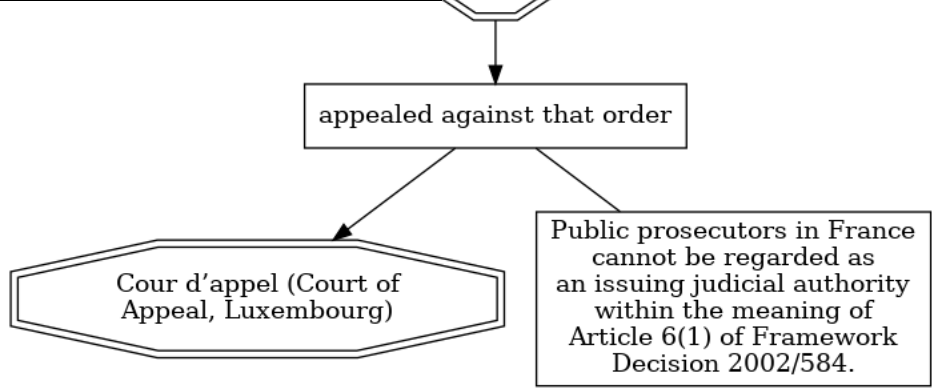

(C) GPT-3.5-Turbo

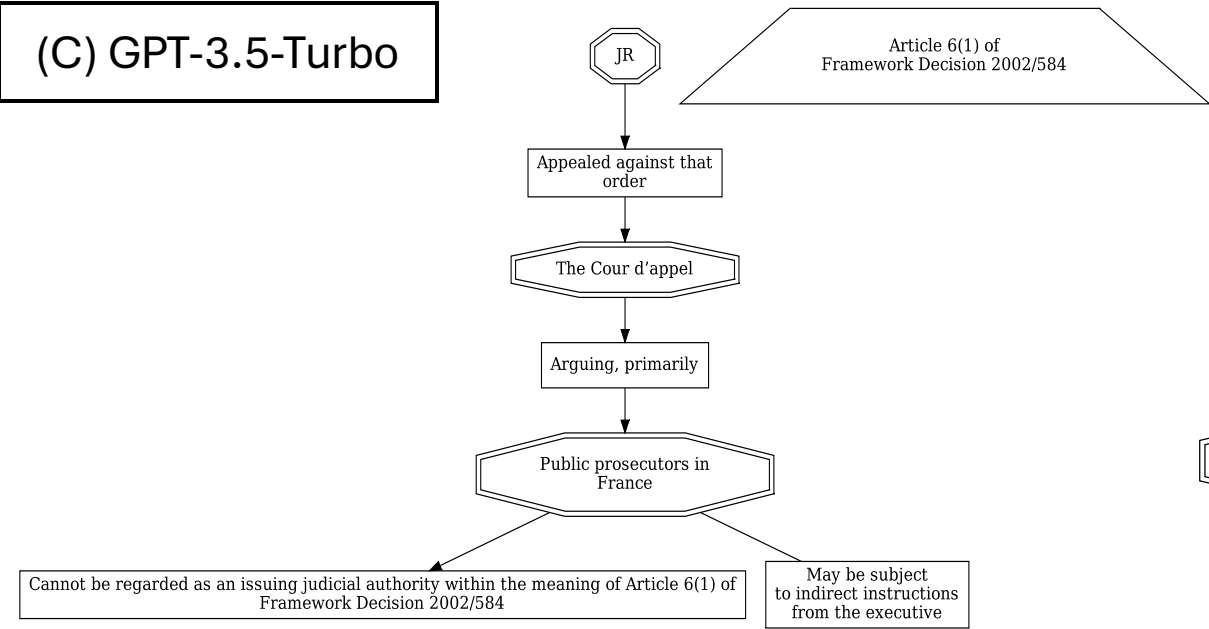

(D) GPT-4

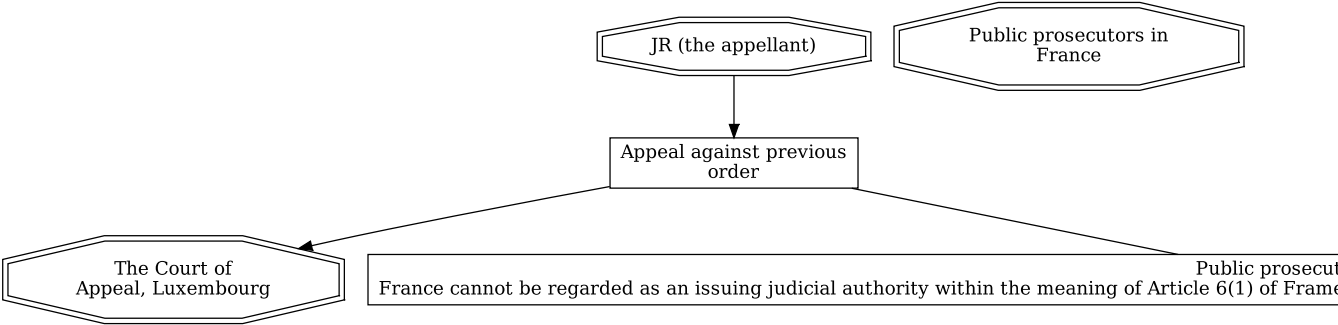

Supplement: Supplementary file 1 [file NAACLAppendix.pdf]
